# Supplementary material for: Toward Trustworthy Neural Program Synthesis
Source: arXiv:2210.00848 source file (2023-10-09)
Supplement: Supplementary file 2 [file appendixexamples.tex]

% \resizebox{\columnwidth}{!}{
% \setlength{\tabcolsep}{20pt}
% \begin{tabular}{m{2cm}| m{2cm} |m{10cm} }
% Prompt & Is program correct  & Generated Program \\
% \hline
% Yes & Yes & \input{appendix_examples/t2} \\
% \hline
% Yes & Yes & \input{appendix_examples/t2} \\
% \hline
% Yes & Yes & \input{appendix_examples/t2} \\
% \end{tabular}
% }

\textbf{Logical Relation Certificates}

\resizebox{\columnwidth}{!}{
\setlength{\tabcolsep}{20pt}
\begin{tabular}{m{7cm}| m{7cm}}
Top 5 Certificates & Random 5 Certificates \\
\hline

\begin{lstlisting}[language=Python, breaklines=true]
import numpy as np
    
def incmatrix(genl1,genl2):
    m = len(genl1)
    n = len(genl2)
    M = None #to become the incidence matrix
    VT = np.zeros((n*m,1), int)  #dummy variable
    
\end{lstlisting}
 &  \\
\hline
 &  \\
\hline
 &  \\
\end{tabular}
}
\subsubsection{MBPP Problem 1}
