# Supplementary material for: Toward Trustworthy Neural Program Synthesis
Source: arXiv:2210.00848 source file (2023-10-09)
Supplement: Supplementary file 3 [file t1.tex]

\begin{lstlisting}[language=Python, breaklines=true]
import numpy as np
    
def incmatrix(genl1,genl2):
    m = len(genl1)
    n = len(genl2)
    M = None #to become the incidence matrix
    VT = np.zeros((n*m,1), int)  #dummy variable
    
\end{lstlisting}
